# Supplementary material for: A Differentiable Integer Linear Programming Solver for Explanation-Based Natural Language Inference
Source: arXiv:2404.02625 source file (2024-04-03)
Supplement: Supplementary file 1 [file appendices.tex]

The pseudo-code to train \textit{Diff-}Comb Explainer end-to-end is summarized in Algorithm~\ref{algo:comb}.

\SetKwComment{Comment}{/* }{ */}
\begin{algorithm}[ht]
\small
\SetAlgoLined
\KwData{$A,~b \gets \textrm{Multi-hop Inference Constraints}$}
\KwData{$f_w \gets \textrm{Graph weight Function}$}
\KwData{$\lambda \gets \textrm{Hyperparameter for DBCS interpolation}$}
% \KwData{$T \gets \textrm{Temperature}$}
$epoch \gets 0$\;
\While{epoch $\leq$ max\_epochs}{
\ForEach {$h_i \in H $}{
$G^i \gets \textrm{fact-graph-construction}(h_i,~F)$\;
$l^i \gets L(h_i,~F)$\;
$\theta \gets clamp([0,~1])$\;
% $embedder \gets STrans(\textrm{pre-trained model})$\;

  $\vec{F} \gets STrans(F)$\;
  $\vec{h_i}  \gets STrans(h_i)$\;
  $s^i \gets S(\vec{h_i},~\vec{F})$\;
  $W^i \gets f_w(s^i,~l^i;~\theta)$\;
  $\hat{Y}^i \gets DBCS(-W^i,~A,~b; \lambda)$\;
  $\gamma^i \gets (W \cdot \hat{Y}^i)\cdot T$\;
}
  $\mathcal{L}_{ans} = l_c(\sigma(\gamma^1,~\gamma^2,~\cdots~\gamma^n),~c_{ans})$\;
  \eIf{$F_{exp}$ is available}{
  $\mathcal{L}_{exp} = l_b(\hat{Y}^{ans}[f_1,~f_2,~\dots,~f_k],~F_{exp})$\;
  $\mathcal{L} = \lambda_{ans}\mathcal{L}_{ans} + \lambda_{exp}\mathcal{L}_{exp}$\;
  }{
    $\mathcal{L} = \mathcal{L}_{ans} $\;
  }
  update $\theta$, $STrans$ using AdamW optimizer by minimizing $loss$\;
  $epoch \gets epoch + 1$\;
}
\KwResult{Store best $\theta$ and $STrans$}
 \caption{\small Training \textit{Diff-}Comb Explainer}
\label{algo:comb}
\end{algorithm}

% The rest of the section details the hyper parameters, code bases and datasets used in our approach to reproduce our experiments.

\paragraph{Experimental Setup:}  We employ the following experimental setup:
\setlist{nolistsep}
\begin{itemize}[noitemsep,leftmargin=*]
    \item \textit{Sentence Transformer Model}: \textsc{all-mpnet-base-v2}~\citep{DBLP:journals/corr/abs-2004-09297}. 
  \item \textit{Fact retrieval representation}:  \textsc{all-mpnet-base-v2} trained with gold explanations of WorldTree Corpus to achieve a Mean Average Precision of 40.11 in the dev-set.
\item \textit{Fact retrieval}: FAISS retrieval~\citep{DBLP:journals/corr/JohnsonDJ17} using pre-cached representations.
\item \textit{Background knowledge}: 5000 abstract facts from the WorldTree table store (WTree) and over 100,000 \textit{is-a} grounding facts from ConceptNet (CNet)~\citep{DBLP:journals/corr/SpeerCH16}.
\item The experiments were carried out for $k=\{1, 2, 3, 5, 10, 20, 30, 40, 50\}$  and the best configuration for each model is selected.
\item The hyperparameters $\lambda, \lambda_{ans},\lambda_{exp},T$ were fine-tuned for 50 epochs using the \href{https://ax.dev/}{Adpative Experimentation Platform}.
\item $M$=2 for ExplanationLP, \textit{Diff-}Explainer and \textit{Diff-}Comb Explainer.
\end{itemize}

\subsection{External code-bases}
\begin{itemize}
    \item Differentiable Blackbox Combinatorial Solvers Examples: \url{https://github.com/martius-lab/blackbox-differentiation-combinatorial-solvers}
    
    \item Sentence Transformer code-base:
    \url{https://huggingface.co/sentence-transformers/all-mpnet-base-v2}
\end{itemize}

\subsection{Integer Linear Programming Optimization}

The components of the linear programming system is as follows:

\begin{itemize}
    \item Solver: Gurobi Optimization \url{https://www.gurobi.com/products/gurobi-optimizer/}
\end{itemize}

\noindent The hyperparatemers used in the ILP constraints:

\begin{itemize}
    \item Maximum number of abstract facts ($M$): 2
\end{itemize}

\noindent Infrastructures used:
\begin{itemize}
    \item CPU Cores: 32
    \item CPU Model: Intel(R) Core(TM) i7-6700 CPU @ 3.40GHz
    \item Memory: 128GB
    % \item OS: Ubuntu 18.04 LTS
\end{itemize}

\subsection{Hyperparameters}

For \textit{Diff-}Comb Explainer we had to fine-tune hyperparameters $\lambda, \lambda_{ans},\lambda_{exp},T$. We fine-tune for 50 epochs using the \href{https://ax.dev/}{Adpative Experimentation Platform} with seed of 42.

The bounds of the hyperparameters are as follows:

\begin{itemize}
    \item $\lambda$: $[100, 300]$
    \item $\lambda_{exp}$: $[0.0, 1.0]$
    \item $\lambda_{ans}$: $[0.0, 1.0]$
    \item $T$: $[1e-2, 100]$
\end{itemize}

The hyperparameters adopted for our approach are as follows:

\begin{itemize}
    \item $\lambda$: 152
    \item $\lambda_{exp}$: 0.72
    \item $\lambda_{ans}$: 0.99
    \item $T$: 8.77
    \item max epochs: 8
    \item gradient accumulation steps: 1
    \item learning rate: 1e-5
    \item weight decay: 0.0
    \item adam epsilon: 1e-8
    \item warmup steps: 0
    \item max grad norm: 1.0
    \item seed: 42
\end{itemize}

The hyperparameters adopted for BERT are as follows:

\begin{itemize}
    \item gradient accumulation steps: 1
    \item learning rate: 1e-5
    \item weight decay: 0.0
    \item adam epsilon: 1e-8
    \item warmup steps: 0
    \item max grad norm: 1.0
    \item seed: 42
    % \item $\lambda$: 6.5
\end{itemize}

We fine-tuned using 4 Tesla V100 GPUs for 10 epochs in total with batch size 32 for $Base$ and 16 for $Large$.

\subsection{Data}
\noindent\textbf{WorldTree Dataset}: Data can be obtained from: \url{http://cognitiveai.org/explanationbank/}
% The 4,400 questions in the WorldTree corpus are split into three different subsets: \emph{train-set} (987), \emph{dev-set} (226), and \emph{test-set} (1,077). 

\noindent\textbf{ARC-Challenge Dataset}: \url{https://allenai.org/data/arc}. Only used the Challenge split.
